# Supplementary material for: Language and Knowledge Representation: A Stratified Approach
Source: arXiv:2504.11492 source file (2025-04-14)
Supplement: Supplementary file 1 [file appendix_c.tex]

\chapter{LIST OF ABBREVIATIONS}
